# Supplementary material for: Computational Indentation in Highly Cross-linked Polymer Networks
Source: arXiv:2202.04065 source file (2022-05-05)
Supplement: Supplementary file 1 [file suppy_materia.pdf]

# Supplementary material "Computational indentation in highly cross-linked polymer networks"

Manoj Kumar Maurya,[1] Céline Ruscher,[2] Debashish Mukherji,[2,*] and Manjesh Kumar Singh[1,†]

[1]*Department of Mechanical Engineering, Indian Institute of Technology Kanpur, Kanpur UP 208016 India*
[2]*Quantum Matter Institute, University of British Columbia, Vancouver BC V6T 1Z4, Canada*

In this supplementary material we provide additional information for some claims made in the main manuscript draft.

## S1. BOND DENSITY PROFILE

The network curing protocol presented in the Main Section IIB reasonably creates a homogeneous sample, see Fig. S1. It can be appreciated that the bonds

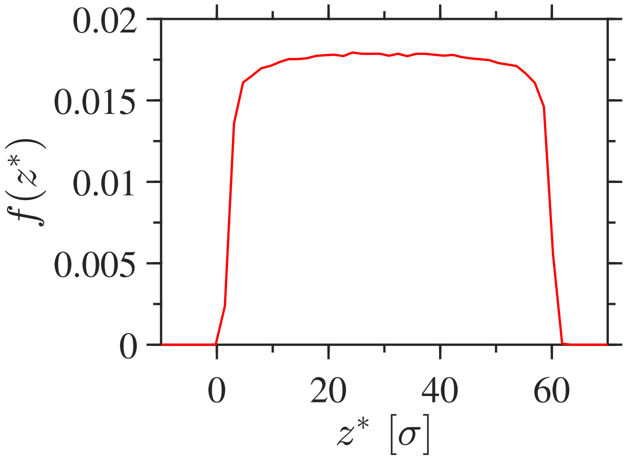


FIG. S1: Bond density $f(z^*)$ along the $z-$direction of the sample, i.e., the direction along which the indentation is applied. The data is shown for a tetrafunctional network.

are rather homogeneous, except near the two interfaces where the confining walls induce the depletion zone.

## S2. MECHANICS DURING LOADING AND UNLOADING

In the Main Fig. 5(a), we have only shown the force $F$ response during unloading starting from tree indentation depths $d$. Here, we show three additional unloading curves, see Fig. S2.

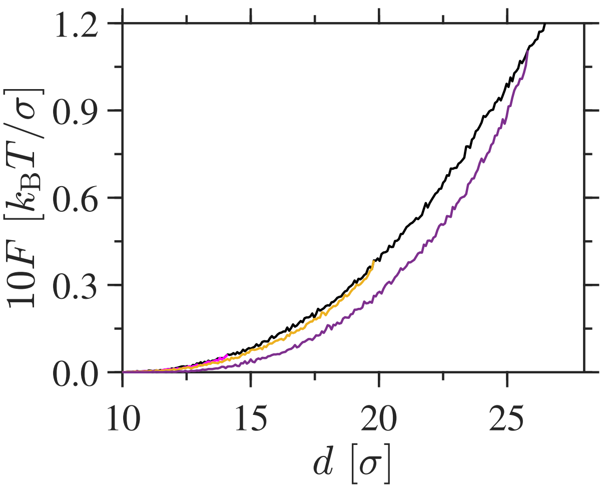


FIG. S2: Force $F$ as a function indentation depth $d$ during three different unloading cycles starting at different $d$. Data is shown for the tetrafunctional network and for an indenter radius $R = 15.0\sigma$. The unloading is performed at a constant unloading velocity $v = 0.005\sigma/\tau$. During the loading cycle, bond breaking starts only around $d \simeq 18.0\sigma$. Therefore, the unloading data starting at $d \simeq 14.0\sigma$ represents the elastic deformation. Note the data here is an extension of the Main text Fig. 5(a).

## S3. FORCE AND STRUCTURAL RELAXATIONS

To monitor the transient relaxations in a system, we have calculated the time evolution of $F$ and the structure as monitored by $d$. To estimate the relaxations, we have performed two different simulations. In the first case, we indent a sample using a velocity $v = 0.05\sigma/\tau$ till the maximum in the force is reached. At this position, the indenter position is fixed and the time evolution of $F$ is monitored. For the relaxation of $d$, we first decouple the indenter from a system and then monitor $d$ with time. The data is shown in Fig. S3.

It can be appreciated that the structural relaxation is about two orders of magnitude faster than the $F$ relaxation. At a first glance this may look rather counter-intuitive because the standard understanding from the dynamic systems, such as the visco-elastic deformation, suggest that the structures relax way slower than the force. Here, however, we observe an opposite trend because we are dealing with an elastic-plastic deformation of a highly cross-linked (HCP) network structure. Fur-

*debashish.mukherji@ubc.ca
†manjesh@iitk.ac.in

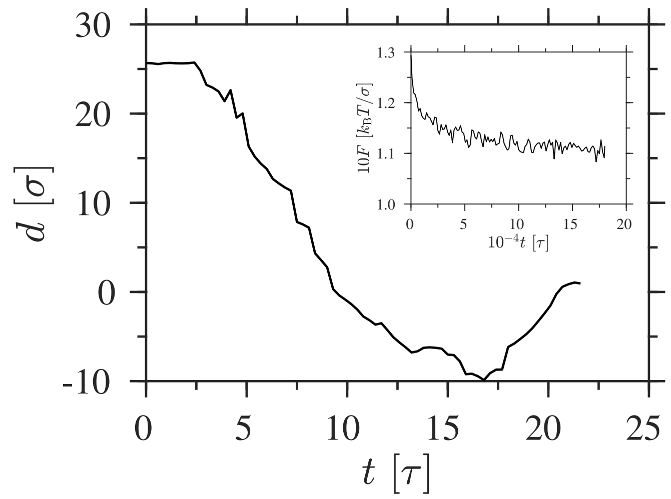


FIG. S3: Main panel shows the temporal relaxations of the depth $d$ and the inset presents relaxation of force $F$. The data is shown for the indenter radius $R = 15.0\sigma$ and for a tetrafunctional network.

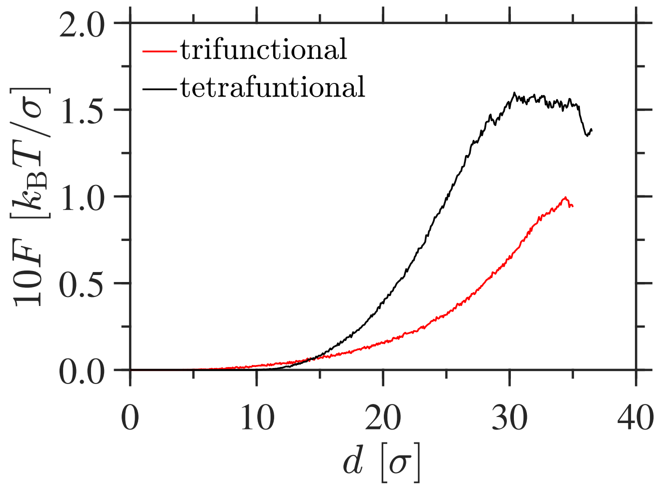


FIG. S4: Force $F$ as a function indentation depth $d$ for two different network functionalities, namely the trifunctional (i.e., $n = 3$) and the tetrafunctional (i.e., $n = 4$) networks. Data is shown for an indenter radius $R = 15.0\sigma$. The indentation is performed at a constant velocity $v = 0.005\sigma/\tau$.

thermore, the HCP network is in its soft gel phase, where a strong restoring force act via the bonded interactions leading to the faster structural relaxation.

## S4. EFFECT OF NETWORK FUNCTIONALITY

In the Main Fig. 6 we have shown the comparative data of two different functionalities with an indenter radius $R = 5.0\sigma$. This is particularly because the small sized indenter can monitor individual bond breaking events. However, we have also calculated the mechanics of both networks using the larger indenter, i.e., for $R = 15.0\sigma$. The corresponding data is shown in Fig. S6. The data is consistent with the generic behavior discussed in the Main Fig. 6. Here, however, force drop events are even less prominent for the trifunctional compared to the data for $R = 5.0\sigma$, see the red data sent in Main Fig. 6.

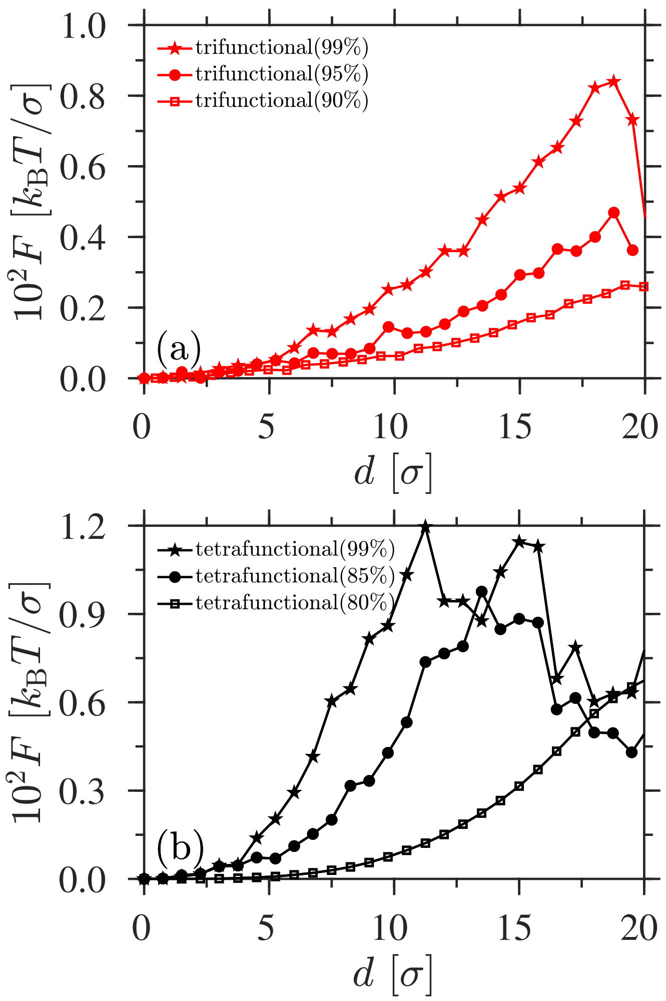


FIG. S5: Force $F$ as a function indentation depth $d$ for two different network functionalities, namely the trifunctional (part a) and the tetrafunctional (part b) networks. Data is shown for three different curing percentages $\mathcal{C}$. Note that for the clarity of presentation, we have only shown the smoothed data.

## S5. EFFECT OF NETWORK CURING PERCENTAGE

As shown in the Main Fig. 7, the network curing percentage $\mathcal{C}$ plays a key role in dictating the predictive mechanical behavior that can serve as an additional tuning parameter. Note that the Main Fig. 7 shows the extracted data from the $F$ versus $d$ curves at different $\mathcal{C}$, see Fig. S5.

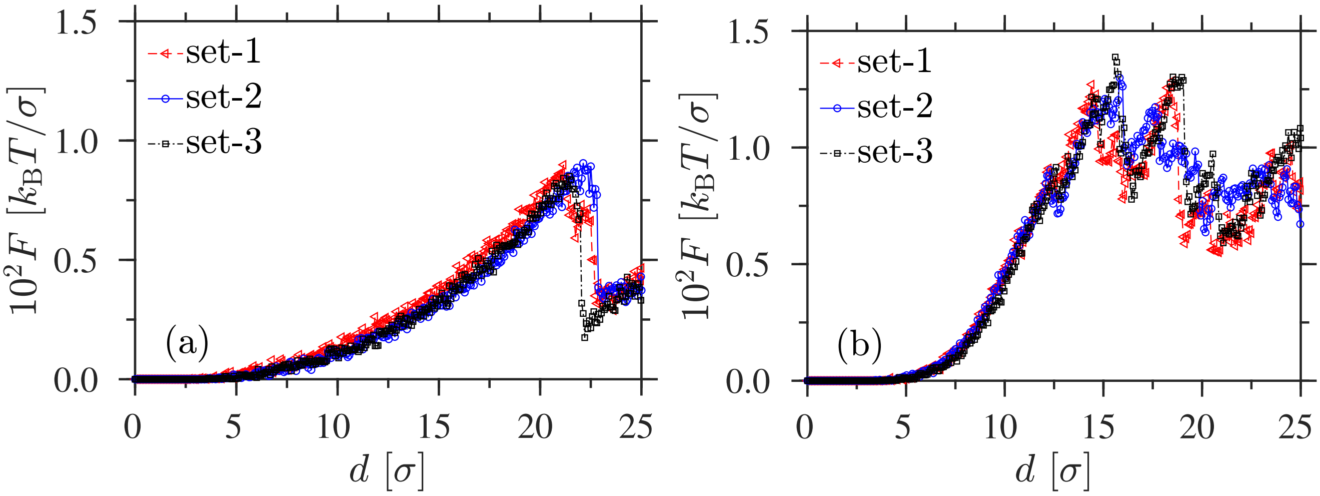


FIG. S6: Force $F$ as a function indentation depth $d$ for the trifunctional (part a) and the tetrafunctional (part b) networks. Data is shown for an indenter radius $R = 5.0\sigma$ and for three different sets. The indentation is performed at a constant velocity $v = 0.005\sigma/\tau$.

## S6. REPRODUCIBILITY OF FORCE-INDENTATION DATA

Most studies of mechanical behavior of polymers are performed within the mid sized simulation domains that many a times induce large error bars. Even when our system sizes are reasonably large consisting of over $2.5 \times 10^5$ particles, we have also performed a set of three different simulations to check if the data are reproduced within the small error. In Fig. S6, the force-indentation curves for $R = 5.0\sigma$ and for both systems are shown. It can be seen that the data is reproduced within 5% error. The error bars for $R = 15.0\sigma$ are even smaller, i.e., about 1% (data not shown).
